# Supplementary material for: NeO 360: Neural Fields for Sparse View Synthesis of Outdoor Scenes
Source: arXiv:2308.12967 source file (2023-08-24)
Supplement: Supplementary file 1 [file 13_additional_quanitative_results.tex]

\section{Additional Quantitative Results:}
\label{sec:add_quantitative_results}

\input{iccv2023AuthorKit/tables/additional_comparisons}

We include additional baseline comparisons with overfitting NeRF baselines~(mipNeRF360~\cite{barron2022mip} and EG3D~\cite{chan2022efficient}) and generalizable NeRF baseline~(SRT~\cite{srt22}). We include these comparisons in Tab.~\ref{tab:add_comparison}. One could clearly observe that naively using triplanes~(Tab.~\ref{tab:add_comparison} row 3, *denotes that we take the triplanar representation without generative losses or training) or local features as in PixelNeRF~(our paper Tab.~\textcolor{red}{4})  hurt the performance. Our method relies on effective combination of local and global features which serves as a strong baseline for the challenging task of 360$^{\circ}$ view synthesis of outdoor scenes. This is further confirmed by our superior results against added baselines~(Tab.~\ref{tab:add_comparison}) and qualitative results~(cf. supp. video). We also include depth reconstruction metrics~(Tab.~\ref{tab:depth_metrics}) and show our techniques' superior results compared to Pixel-NeRF.

\textbf{Difference from~\textit{EG3D} and~\textit{GAUDI}:} Both approaches are generative models which use adversarial losses for training and GAUDI uses GAN inversion for conditional synthesis. Our approach, NeO 360, does not rely on expensive GAN inversion and directly outputs density/RGB for all test views. Motivated by your excellent comments, we add a baseline~(Tab.~\ref{tab:add_comparison} row 3) comparing EG3D/GAUDI's representation i.e. triplanes which reduces to a vanilla NeRF variant optimized per scene. We leave the generative counterpart comparisons to future work and hope our dataset is a useful to the community in that direction.
